# Supplementary material for: Graph Contrastive Learning with Implicit Augmentations
Source: arXiv:2211.03710 source file (2022-11-07)
Supplement: Supplementary file 1 [file 6Appendix.tex]

\section{Algorithm}
We demonstrate the learning algorithm for iGCL at node-level in Algorithm~\ref{alg algorithm}. Different from graph-level, after generating embeddings from the backbone and projection, we randomly sample $b$ node embeddings for contrastive learning, due to the memory constraint.
\begin{algorithm}[h]
\caption{iGCL for Node-level Task} \label{alg algorithm}
\textbf{Input}: Graph $\mathcal{G}$ with $N$ nodes; Graph Auto-Encoder $VGAE(\cdot)$; GNN backbone $\mathcal{F}(\cdot)$ and projection head $\mathcal{P}(\cdot)$.\\
\textbf{Parameter}: $\Phi$ in $VGAE(\cdot)$; $\Theta$ in $\mathcal{F}(\cdot)$ and $\mathcal{P}(\cdot)$.\\
\vspace{-1.2em}
\begin{algorithmic}[1] %[1] enables line numbers
\FOR{$epoch = 1,\cdots,T$}
    \STATE Generate ${\bm \mu}_n, {\bm \sigma}_n$ for $\mathcal{G}_n$ from $VGAE$.
    \FOR{$k = 1,\cdots, K$}
        \STATE Update $\Phi$ by $\nabla \mathcal{L}_{VGAE}$.
    \ENDFOR
    \STATE Generate ${\bm z}_n$ for $v_n$ from $\mathcal{F}(\cdot)$ and $\mathcal{P}(\cdot)$.
    \STATE Sample a batch of size $b$ from $\{z_n\}_{n=1}^N$
    \STATE Update $\Theta$ by $\nabla \mathcal{L}_{upper}$.
\ENDFOR
\STATE \textbf{return} Embedding $\bf Z$ from the optimized $\mathcal{F}(\cdot)$.
\end{algorithmic}
\end{algorithm}

\section{Experimental Details}
In this section, we present the details of dataset statistics and hyper-parameter settings for reproduction, as shown in Table~\ref{tab Graph stats} (Graph-level) and Table~\ref{tab Node stats} (Node-level) below. All models are implemented with PyTorch 1.10.0 \cite{paszke2019pytorch} and PyTorch Geometric 2.0.4 \cite{fey2019fast}. The experiments are conducted on 8 NVIDIA Tesla V100S GPUs with 32GB memory and two Intel Xeon CPUs.

\subsection{General Settings}
We initialize our GNN backbones and projection heads with Glorot initialization \cite{glorot2010understanding} and use Adam \cite{kingma2014adam} as the optimizer, where the learning rate $lr$ and weight decay $\ell_2$ are chosen from \{$5\times10^{-4}$, $10^{-4}$\} and $\{10^{-2}, 5\times10^{-3}, 10^{-3}, 5\times10^{-4}\}$. The VGAE is trained with the default settings from the original paper \cite{kipf2016variational}, that is, using Adam optimizer with a learning rate of 0.01 and no weight decay. 

\subsection{Graph-level Settings}
At graph level, we use GIN \cite{xu2019powerful} as the model's backbone for all datasets and use a linear projection head with optional skip-connection. The number of epochs, backbone layers, batch size and embedding size are chosen from \{20, 60, 100\}, \{2, 5, 8\} , \{16, 32, 64, 128\} and \{128, 256, 512\}. We select $\tau$ by tuning from range [0.01, 10]. At testing stage, we report the mean accuracy from 10-fold cross-validation with a SVM classifier applied to the learned embeddings, where $C$ is chosen from $\{10^{-3}, 10^{-2}, \cdots,10^{3}\}$.

\subsection{Node-level Settings}
We use 2-layer GCN or GAT as the GNN backbone for node-level tasks. The embedding size is are chosen from \{128, 256, 512\}, and the temperature $\tau$ is tuned from [0.01, 5]. After contrastive learning, we train an independent logistic regression for classification. For testing, we select epochs with top 5 validation accuracy and average the weights to generate final predictions.

%--------------------------------Graph Level---------------------------------------
\linespread{1.2}
\begin{table*}[t]
\centering
\resizebox{0.99\textwidth}{!}{
\begin{tabular}{c | l c c c c c c }
    \hline\hline
    \textbf{Graph} & \textbf{Dataset}  & \textbf{MUTAG} & \textbf{NCI1} & \textbf{PROTEINS} & \textbf{COLLAB} & \textbf{IMDB-B} & \textbf{IMDB-M}\\
    \hline\hline
    \multirow{5}{*}{\textbf{Statistics}} 
    & Type         & Molecule & Molecule & Molecule & Social & Social & Social \\
    & \# Graphs    & 188 & 4,110 & 1,113 & 5,000 & 1,000 & 1,500 \\
    & \# Classes   & 2 & 2 & 2 & 3 & 2 & 3\\
    & Avg. Nodes   & 17.9 & 29.9 & 39.1 & 74.5& 19.8 & 13.0 \\
    & Avg. Edges   & 19.8 & 32.3 & 72.8 & 2,457.8 & 96.5 & 65.9\\
    \hline
    \multirow{6}{*}{\textbf{Settings}}
    & Projection  & Skip & Linear & Linear & Linear & Linear & Skip \\
    & num\_epochs & 100 & 100 & 20 & 20 & 20 & 100\\
    & num\_layers & 5 & 5 & 2 & 8 & 2 & 8\\
    & emb\_size   & 256 & 256 & 256 & 256 & 512 & 128 \\
    & batch\_size & 16 & 32 & 64 & 128 & 16 & 64\\
    & $lr$        & $5\times10^{-4}$ & $10^{-4}$ & $10^{-4}$ & $5\times10^{-4}$ & $10^{-4}$ & $5 \times 10^{-4}$ \\
    & $\ell_2$    & $5\times 10^{-3}$ & $5\times 10^{-3}$ & $10^{-2}$ & $10^{-2}$ & $5\times10^{-3}$ & $10^{-2}$ \\
    & $\tau$      & 0.01 & 3.54 & 5 & 1.98 & 5.0 & 10.0 \\
    \hline\hline
\end{tabular}}
\caption{Dataset statistics and hyper-parameter settings for Graph-level task.}
\label{tab Graph stats}
\end{table*}

%--------------------------------Node Level---------------------------------------
\begin{table*}[t]
\centering
\resizebox{0.99\textwidth}{!}{
\begin{tabular}{c | l c c c c c }
    \hline\hline
    \textbf{Node} & \textbf{Dataset}  & \textbf{Cora} & \textbf{Citeseer} & \textbf{PubMed} & \textbf{Photo} & \textbf{Computers}\\
    \hline\hline
    \multirow{5}{*}{\textbf{Statistics}} 
    & Type         & Citation & Citation & Citation & Amazon Sales & Amazon Sales \\
    & \# Features  & 1,433 & 3,703 & 500 & 745 & 767\\
    & \# Classes   & 7 & 6 & 3 & 8 & 10\\
    & \# Nodes     & 2,708 & 3,327 & 19,717 & 7,650 & 13,752\\
    & \# Edges     & 5,429 & 4,732 & 44,338 & 119,081 & 245,861\\
    \hline
    \multirow{6}{*}{\textbf{Settings}}
    & Backbone  & GCN & GAT & GCN & GAT & GAT \\
    & num\_epochs & 300 & 300 & 1000 & 600 & 600 \\
    & emb\_size   & 256 & 512 & 128 & 256 & 256 \\
    & dropout   & 0.5 & 0.5 & 0.5 & 0.5 & 0.5 \\
    & $lr$ & $10^{-4}$ & $5\times10^{-4}$ & $10^{-4}$ & $5\times10^{-3}$ & $10^{-3}$ \\
    & $lr$ step & - & 0.85 & - & 0.85 & 0.85 \\
    & $\ell_2$ & $5\times 10^{-3}$ & $10^{-2}$ & $10^{-4}$ & $5\times 10^{-3}$ & $5\times 10^{-3}$ \\
    & $\tau$ & 1.0 & 5.0 & 4.7 & 1.0 & 1.0 \\
    \hline\hline
\end{tabular}}
\caption{Dataset statistics and hyper-parameter settings for Node-level task.}
\label{tab Node stats}
\end{table*}
